# Supplementary material for: Scientific Machine Learning for Modeling and Simulating Complex Fluids
Source: arXiv:2210.04431 ancillary file (2022-10-10)
Supplement: Supplementary file 1 [file RUDEs_SI__arXiv_.pdf]

Supplemental Material:

# Scientific Machine Learning for Complex Fluid Modeling

Kyle R. Lennon[1], Gareth H. McKinley[2], and James W. Swan[1]

[1]*Department of Chemical Engineering, Massachusetts Institute of Technology, Cambridge, MA 02142*

[2]*Department of Mechanical Engineering, Massachusetts Institute of Technology, Cambridge, MA 02139*

## Hydrogel Linear Rheology

A small amplitude oscillatory shear frequency sweep was performed on the DHR-3 rheometer (8mm parallel place, 25°C) to characterize the linear mechanical response of the hydrogel system. The experiment was conducted in stress control with a fixed amplitude of $\sigma_0 = 5$ Pa, with frequencies ranging from 100 rad/s to 1 rad/s (five frequencies per decade). The storage and loss moduli computed from these experiments are presented as circles in Figure S1. The linear response was fit to a single linear Maxwell mode:

$$G^*(\omega) = \frac{G_0(i\omega\tau_1)}{1 + i\omega\tau_1}, \tag{S1}$$

by least squares regression, from which the optimal values of $G_0 = 37585$ Pa and $\tau_1 = 0.557$ s were obtained. The resulting best fit to the data are shown by the dashed lines in Figure S1.

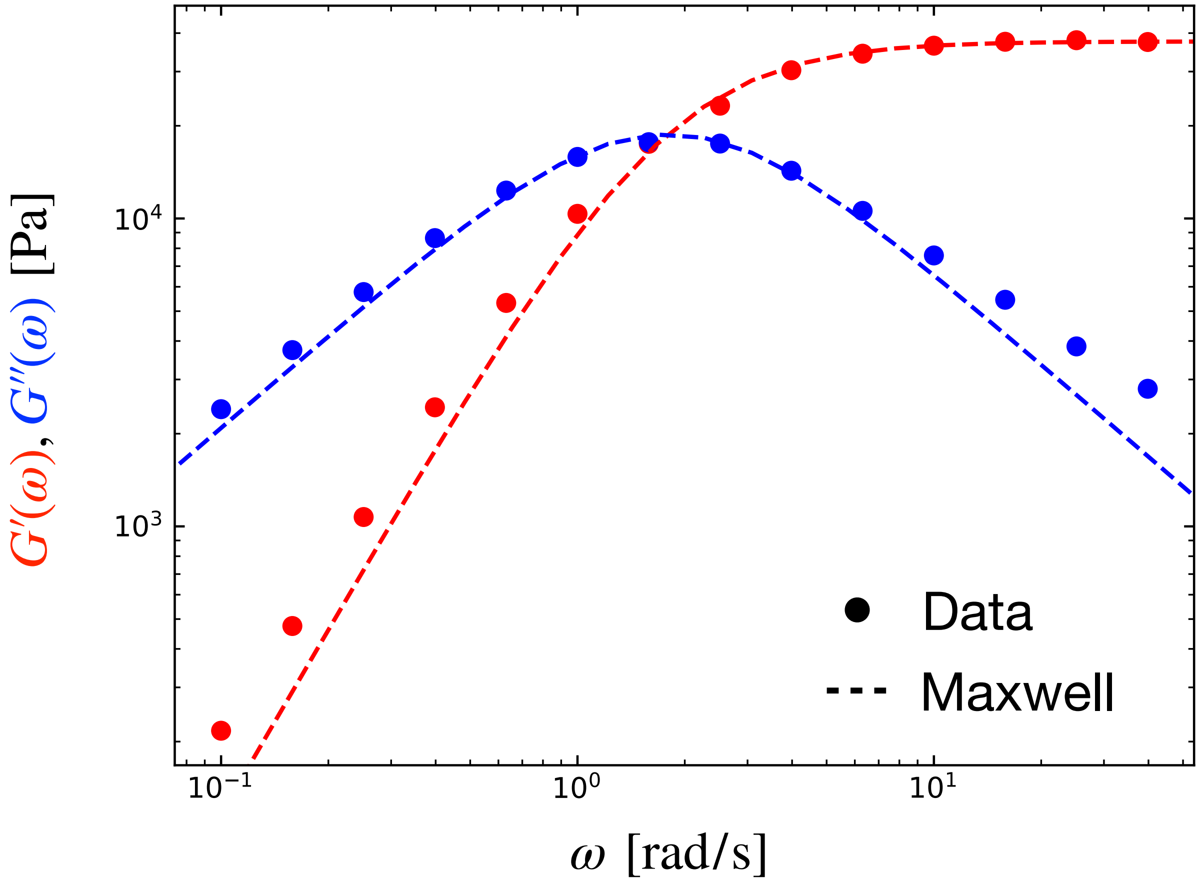


Figure S1: The linear mechanical response of the metal-crosslinked polymer hydrogel system. The measured storage ($G'(\omega)$) and loss ($G''(\omega)$) moduli are shown by red and blue symbols, respectively. The corresponding best-fit predictions of the single-mode Maxwell model ($G_0 =$ 37585 Pa and $\tau_1 = 0.557$ s) are shown by dashed lines.
